# Supplementary material for: Efficient Calculation of Excitonic Effects in Solids Including Approximated Quasiparticle Energies
Source: arXiv:2003.11968 source file (2020-03-26)
Supplement: Supplementary file 1 [file supp-material-PRBformat.pdf]

# Supplemental Material for: Efficient Calculation of Excitonic Effects in Solids Including Approximated Quasiparticle Energies

Filipe Matusalem, Marcelo Marques, Ivan Guilhon, and Lara K. Teles
*Grupo de Materiais Semicondutores e Nanotecnologia (GMSN),*
*Instituto Tecnológico de Aeronáutica (ITA), 12228-900 São José dos Campos/SP, Brasil*

## I. OPTICAL PROPERTIES

In Fig. S1 is show the imaginary part of dielectric function calculated using hybrid HSE and DFT-1/2 methods for comparison.

---

[1] Aspnes D E and Studna A A 1983 *Phys. Rev. B* **27** 985–1009

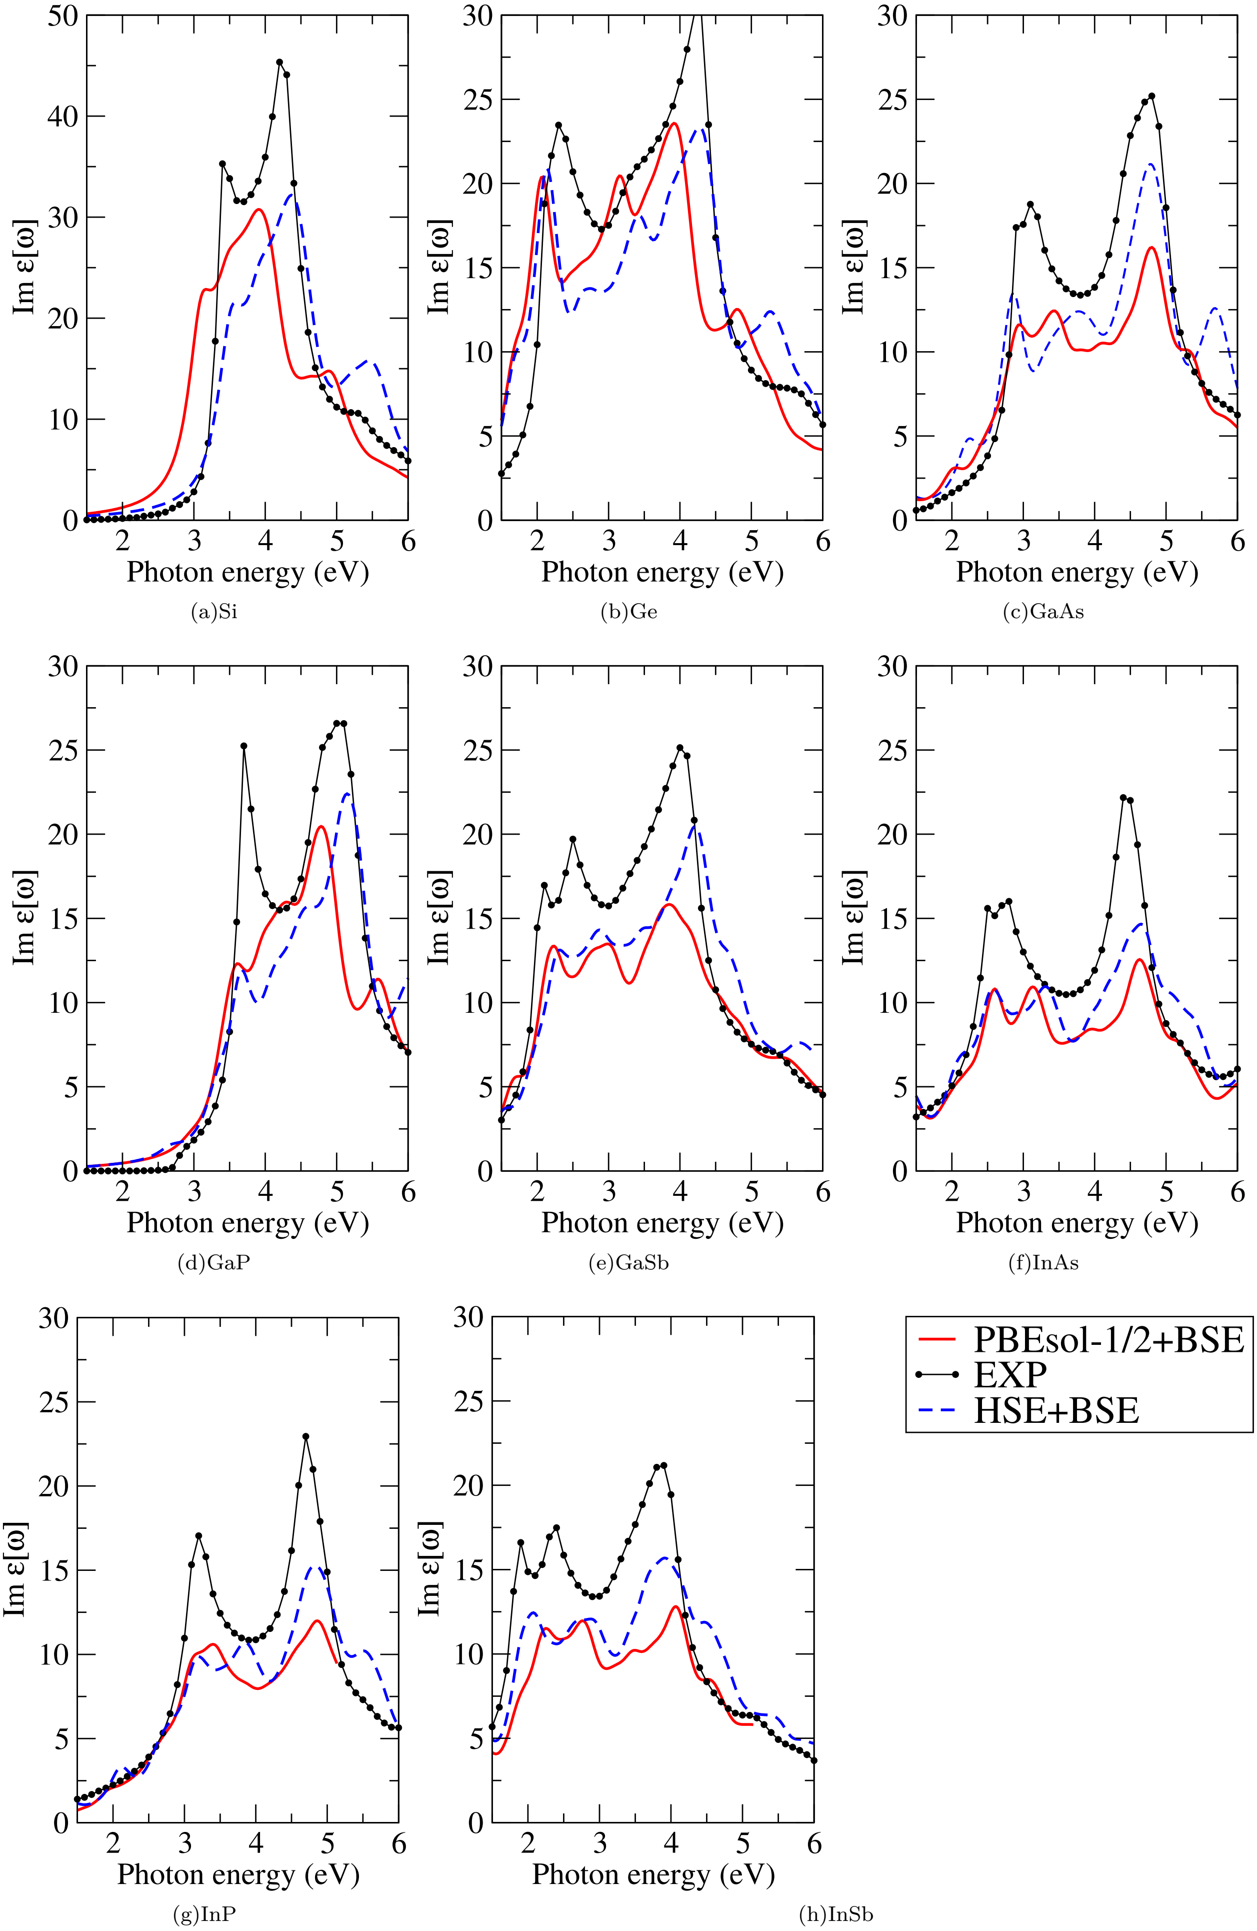


(a)Si (b)Ge (c)GaAs (d)GaP (e)GaSb (f)InAs (g)InP (h)InSb

FIG. S1: (Color online) Imaginary part of dielectric function. Blue dotted curve: HSE+BSE. Red continuous curve: PBEsol-1/2 + BSE. Black line-Dots curve: experiment[1].
